# Supplementary material for: OmniXAS: A Universal Deep-Learning Framework for Materials X-ray Absorption Spectra
Source: arXiv:2409.19552 ancillary file (2025-04-15)
Supplement: Supplementary file 1 [file supplementary.pdf]

# Supplementary Materials:
# "OmniXAS: A Universal Deep-Learning Framework for Materials X-ray Absorption Spectra"

Shubha R. Kharel,[1,*] Fanchen Meng,[2] Xiaohui Qu,[2] Matthew R. Carbone,[1,†] and Deyu Lu[2,‡]

[1] *Computing and Data Sciences Directorate, Brookhaven National Laboratory, Upton, New York 11973, USA*
[2] *Center for Functional Nanomaterials, Brookhaven National Laboratory, Upton, New York 11973, USA*

(Dated: April 10, 2025)

## I. STARTING ENERGY POINTS OF XANES SPECTRA

| Element | $E_{\text{start}}$ (eV) |
|---|---|
| Co | 7709.282 |
| Cr | 5989.168 |
| Cu | 8983.173 |
| Fe | 7111.23 |
| Mn | 6537.886 |
| Ni | 8332.181 |
| Ti | 4964.504 |
| V | 5464.097 |

TABLE S1. Starting energy points for each element considered in the dataset. All spectra span a 35 eV energy range and are sampled on a 0.25 eV uniform grid.

## II. DATA PROCESSING

| Element | Total Spectra | Unconverged | Anomalies | ML Data |
|---|---|---|---|---|
| Ti | 8,973 | 149 | 2,402 | 6,422 |
| V | 15,498 | 801 | 3,884 | 10,813 |
| Cr | 6,665 | 2,617 | 981 | 3,067 |
| Mn | 21,418 | 1,843 | 2,521 | 17,052 |
| Fe | 17,605 | 2,853 | 2,685 | 12,067 |
| Co | 14,902 | 1,431 | 2,718 | 10,753 |
| Ni | 5,743 | 408 | 1,000 | 4,335 |
| Cu | 5,520 | 221 | 1,127 | 4,172 |
| Ti (VASP) | 3,941 | 0 | 157 | 3,784 |
| Cu (VASP) | 3,242 | 0 | 16 | 3,226 |

TABLE S2. Number of spectra used in the study

* skharel@bnl.gov
† mcarbone@bnl.gov
‡ dlu@bnl.gov

## III. DETAILS OF THE MLP IN THE XAS BLOCK

- Linear layers form the backbone of the MLP, enabling the network to learn complex mappings between input and output spaces:

$$\text{Linear}_l(\mathbf{h}) = W_l\mathbf{h} + \mathbf{b}_l. \tag{1}$$

Here, the weight matrix, $W_l$, and bias vector, $\mathbf{b}_l$, are learnable parameters that the network adjusts during training to capture the underlying patterns in the data.

- Batch normalization plays a crucial role in stabilizing the training process. By standardizing the inputs to each layer, it helps mitigate the internal covariate shift problem, allowing for faster and more stable training [1].

- The SiLU activation function introduces non-linearity into the network, which is essential for capturing complex relationships. SiLU has been shown to outperform ReLU in many scenarios [2]:

$$\text{SiLU}(\mathbf{x}) = \mathbf{x} \odot \sigma(\mathbf{x}), \tag{2}$$

where $\sigma(\mathbf{x}) = (1 + e^{-\mathbf{x}})^{-1}$ is the element-wise sigmoid function and $\odot$ is the element-wise product. The smooth nature of SiLU aids in the propagation of gradient during training.

- Dropout serves as a powerful regularization step, preventing overfitting by randomly deactivating a fraction of nodes during training. This encourages the network to learn more robust features and reduces its reliance on any single node [3]. We set dropout rate of 0.5 for all Dropout layers in XAS-block.

- The Softplus activation in the final layer ensures that the output respects the physical constraints of XAS spectra:

$$\text{Softplus}(\mathbf{x}) = \log(1 + e^{\mathbf{x}}), \tag{3}$$

where all operations are applied element-wise. This function guarantees positive outputs, which is crucial as XAS intensities cannot be negative.

## IV. HYPER-PARAMETER OPTIMIZATION

We used Bayesian optimization with a Tree-Structured Parzen Estimator (TPE) sampler [4] to determine the optimal set of MLP architecture and training parameters utilizing the Optuna package [5]. This apprach efficiently explores the hyperparameter space, resulting in an optimal configuration for the model's widths, depths, and batch sizes.

| **Parameter** | **Range** | **Step** |
|---|---|---|
| Width | 100 – 800 | 50 |
| Depth | 1 – 4 | 1 |
| Batch Sizes | $2^6$, $2^7$, $2^8$, $2^9$ | |

TABLE S3. Search space for hyperparameter optimization

| **Model** | **Element** | **Optimal Batch Size ($2^x$)** | **Layer Widths** |
|---|---|---|---|
| Compound-specific FEFF | Co | 32 | 64 → 600 → 550 → 450 → 141 |
| | Cr | 32 | 64 → 450 → 350 → 150 → 141 |
| | Cu | 32 | 64 → 600 → 600 → 400 → 141 |
| | Fe | 64 | 64 → 450 → 400 → 450 → 141 |
| | Mn | 64 | 64 → 500 → 400 → 300 → 141 |
| | Ni | 32 | 64 → 600 → 300 → 141 |
| | Ti | 64 | 64 → 600 → 600 → 450 → 141 |
| | V | 32 | 64 → 600 → 550 → 450 → 141 |
| Universal FEFF | ALL | 64 | 64 → 500 → 500 → 550 → 141 |
| Compound-specific VASP | Ti | 32 | 64 → 500 → 600 → 400 → 141 |
| | Cu | 64 | 64 → 550 → 600 → 400 → 141 |

TABLE S4. All optimal model architectures and training parameters used in this work.

## V. LOCAL STRUCTURE REPRESENTATION

### A. Atom-Centered Symmetry Function (ACSF)

The ACSF descriptors [6] (via the DScribe package [7]) used in this work are summarized in the Supplemental Information of Ref. [8]. ACSF parameters (chosen to be the same as those used in Ref. [9]) are shown in Table V A.

```
r_cut: 6.0 (Angstroms)
g2_params
    [1.00, 0.00]
    [0.10, 0.00]
    [0.01, 0.00]
g4_params
    [0.001, 1.0, -1.0]
    [0.001, 2.0, -1.0]
    [0.001, 4.0, -1.0]
    [0.010, 1.0, -1.0]
    [0.010, 2.0, -1.0]
    [0.010, 4.0, -1.0]
    [0.100, 1.0, -1.0]
    [0.100, 2.0, -1.0]
    [0.100, 3.0, -1.0]
```

TABLE S5. ACSF parameters used in for DScribe[7] package.

### B. Smooth Overlap of Atomic Position (SOAP)

The SOAP descriptors [10] (also via the DScribe package [7]) used in this work are also summarized in the Supplemental Information of Ref. [8]. SOAP parameters are shown in Table S6.

| $R_C$ (Å) | $n_{max}$ | $l_{max}$ | $\sigma$ | rbf |
|---|---|---|---|---|
| 6.0 | 3 | 3 | 1.0 | gto |

TABLE S6. SOAP parameters

# VI. EXAMPLE PREDICTIONS

## A. ExpertXAS

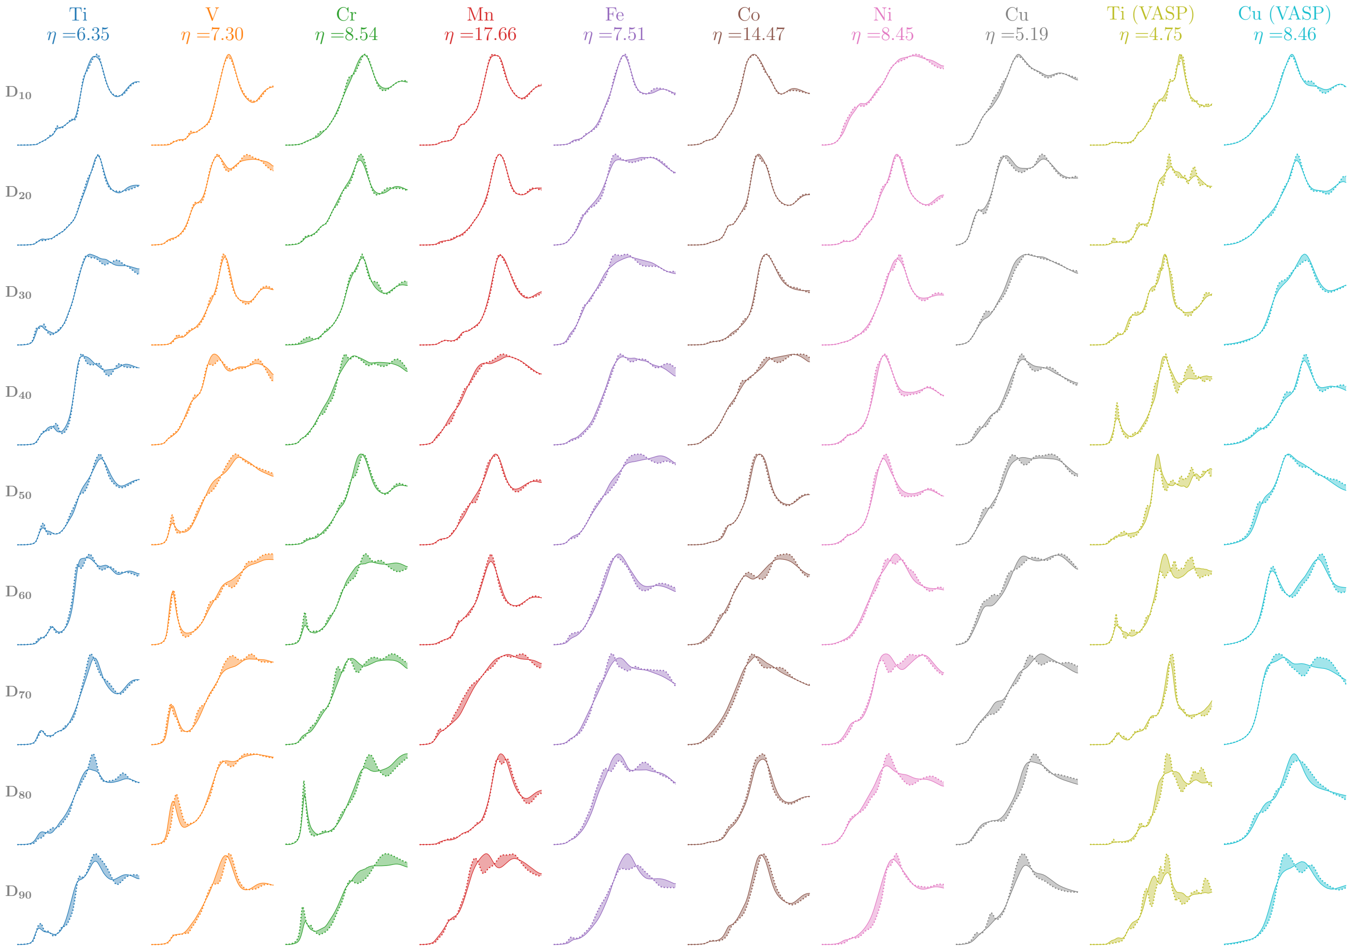


FIG. S1. Example Predictions form ExpertXAS model at deciles of the MSE-per-spectrum distribution.

## B. UniversalXAS

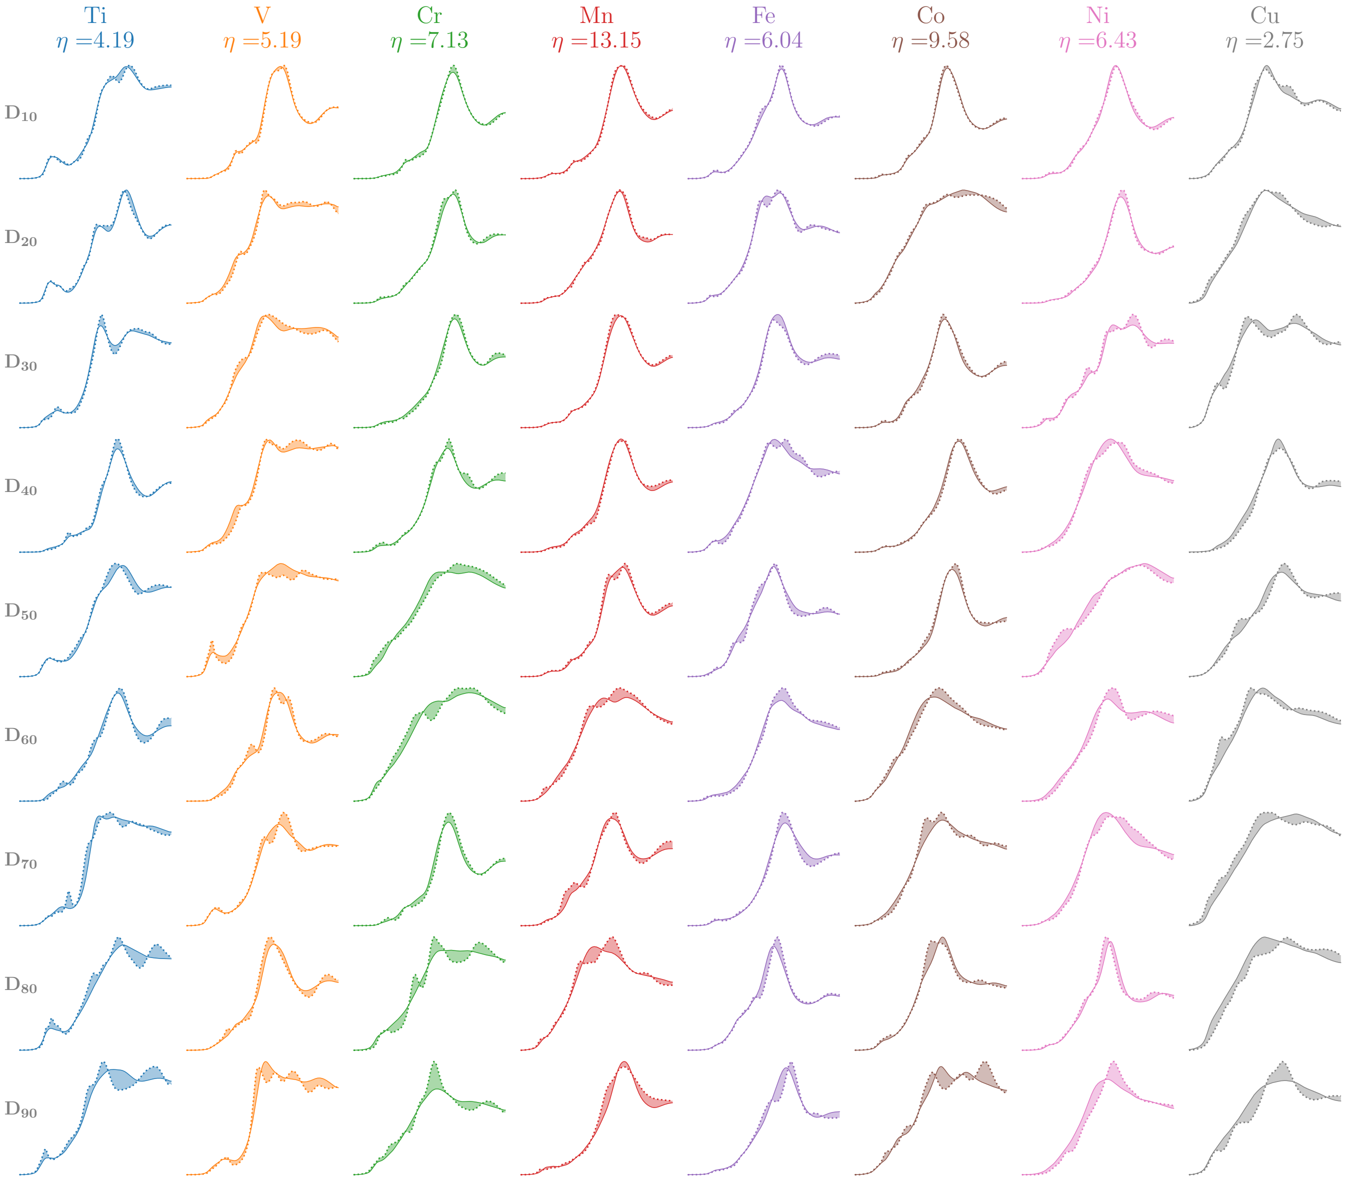


FIG. S2. Example Predictions form UniversalXAS model at deciles of the MSE-per-spectrum distribution.

### C. Tuned-UniversalXAS

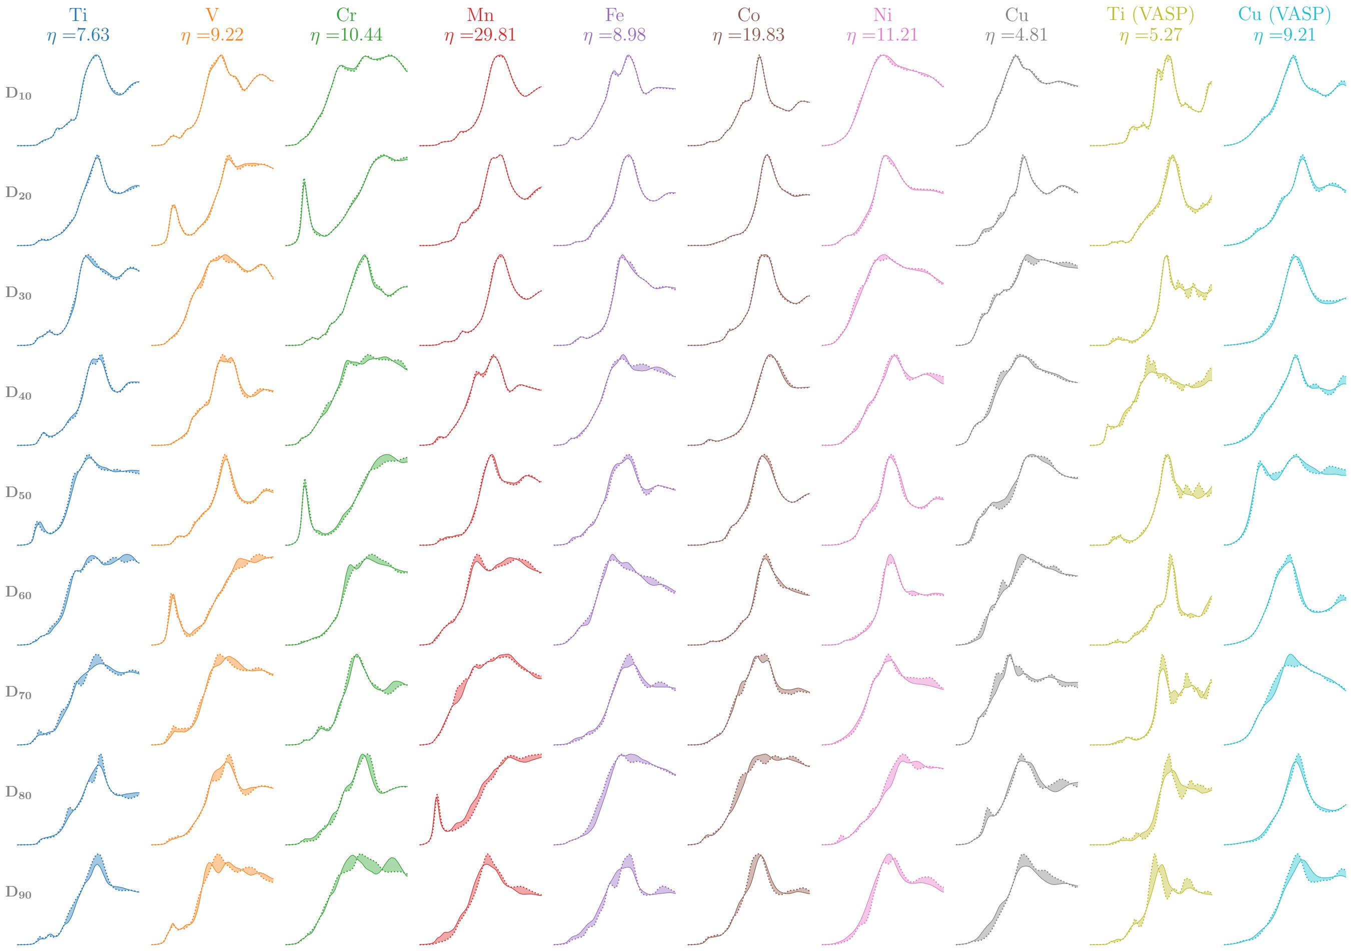


FIG. S3. Example Predictions form RefinedXAS model at deciles of the MSE-per-spectrum distribution.

## VII. MODEL PERFORMANCES VS TRANSFER-LEARNING STRATEGY

### A. Principal Component Analysis

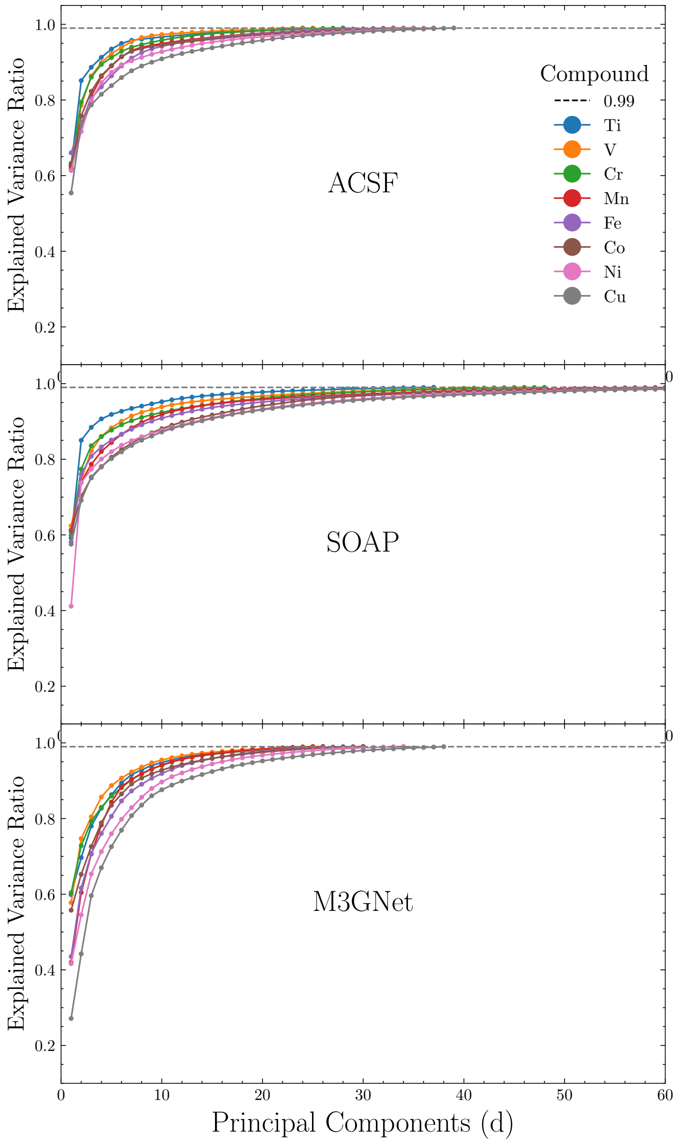


FIG. S4. Explained variance of the PCA decomposition of features

## B. Traditional Featurization vs Transfer-Feature

| | ACSF | | | SOAP | | | Transfer-feature | | |
|---|---|---|---|---|---|---|---|---|---|
| Element | LinReg | GBR | MLP | LinReg | GBR | MLP | LinReg | GBR | MLP |
| Ti | 1.452 | 1.552 | 1.178 | 1.691 | 1.690 | 1.251 | 3.117 | 3.042 | **6.348** |
| V | 1.257 | 1.291 | 1.362 | 1.245 | 1.387 | 1.397 | 3.729 | 4.046 | **7.304** |
| Cr | 1.673 | 1.630 | 1.264 | 1.728 | 1.657 | 1.250 | 5.352 | 4.718 | **8.536** |
| Mn | 2.020 | 2.256 | 2.318 | 2.186 | 2.241 | 2.575 | 8.551 | 8.853 | **17.664** |
| Fe | 1.412 | 1.462 | 1.568 | 1.465 | 1.463 | 1.693 | 3.637 | 3.644 | **7.510** |
| Co | 1.595 | 1.634 | 1.536 | 1.637 | 1.593 | 1.702 | 5.036 | 4.942 | **14.468** |
| Ni | 1.515 | 1.528 | 1.587 | 1.593 | 1.533 | 1.711 | 4.435 | 3.207 | **8.447** |
| Cu | 1.213 | 1.167 | 1.272 | 1.200 | 1.153 | 1.340 | 2.537 | 1.839 | **5.193** |

TABLE S7. Performance ($\eta$) of the Linear Regression (LinReg), Gradient Boosting Regressor (GBR), and Multi-Layer Perceptron (MLP) models trained with the ACSF, SOAP, and transfer-features. Best performance is highlighted in bold. MLP models correspoinds to the XAS-block in ExpertXAS models.

## VIII. BASELINE MODEL PERFORMANCES

| Element | Baseline MSE |
|---|---|
| Ti | 0.0386 |
| V | 0.0402 |
| Cr | 0.0357 |
| Mn | 0.0400 |
| Fe | 0.0234 |
| Co | 0.0194 |
| Ni | 0.0205 |
| Cu | 0.0105 |
| Ti VASP | 0.1566 |
| Cu VASP | 0.0234 |

TABLE S8. Median MSE of the baseline models which predicts the average of the training data.

## IX. REGULARIZATION DURING FINETUNING

TABLE S9. Performance metric ($\eta$) comparison between ExpertXAS and tuned-UniversalXAS models with different Dropout configurations during fine-tuning. Two settings were tested: active Dropout (rate=0.5) and disabled Dropout (rate=0). In the main text, presented results follow a mixed approach where Dropout was deactivated for element-specific FEFF datasets but kept active for VASP datasets.

| Element | ExpertXAS | Fine-tuned UniversalXAS | |
|---|---|---|---|
| | $\eta$ | $\eta$ (Dropout=0.5) | $\eta$ (Dropout=0) |
| Ti | 6.35 | 7.01 | 7.63 |
| V | 7.30 | 8.07 | 9.22 |
| Cr | 8.54 | 10.69 | 10.44 |
| Mn | 17.66 | 21.52 | 29.81 |
| Fe | 7.51 | 8.92 | 8.98 |
| Co | 14.47 | 16.06 | 19.83 |
| Ni | 8.45 | 10.78 | 11.21 |
| Cu | 5.19 | 5.18 | 4.81 |
| Ti VASP | 4.75 | 5.27 | 4.68 |
| Cu VASP | 8.46 | 9.21 | 8.83 |

## X. NEURAL SCALING

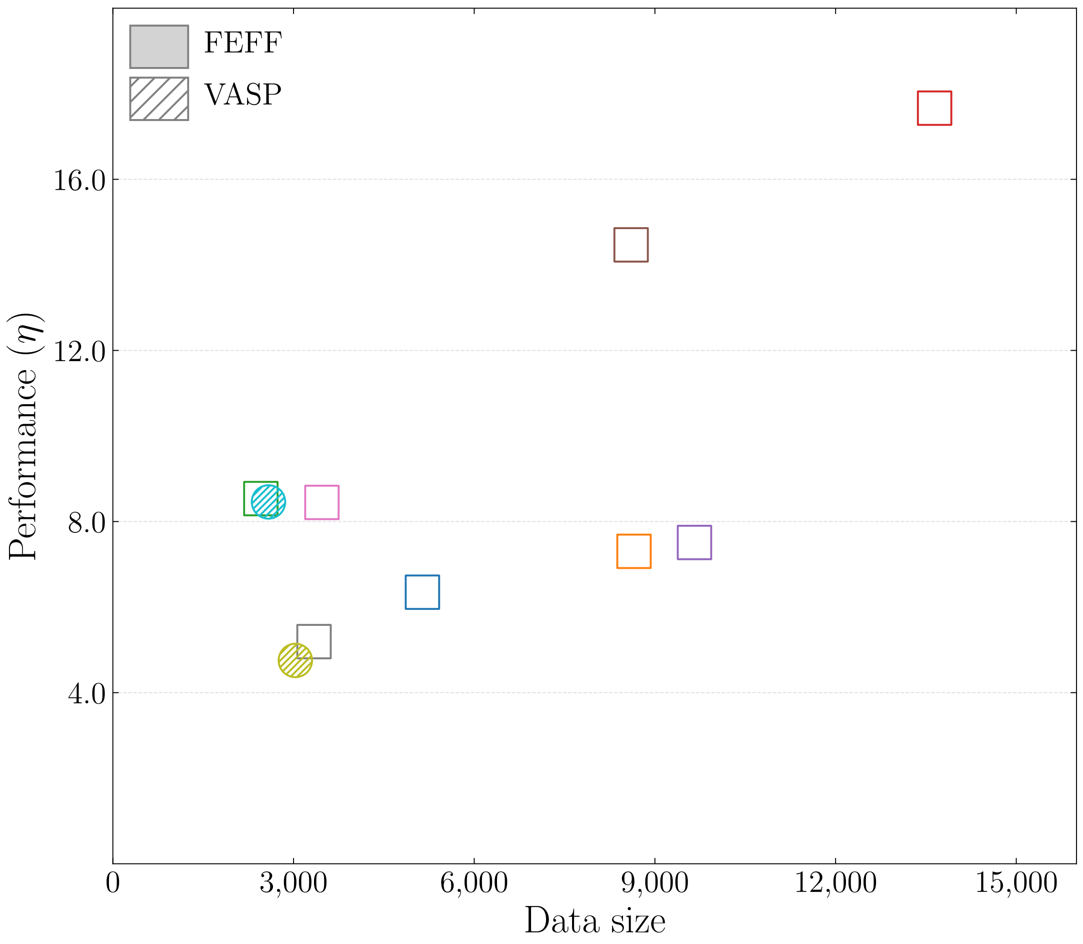


FIG. S5. The model performance is plotted against the quantity of training data provided solely for illustrative purposes, as it disregards the complexity of the data, model sizes, and other factors associated with neural scaling law.[11].

## XI. STATISTICAL SIGNIFICANCE OF THE PERFORMANCE DIFFERENCE

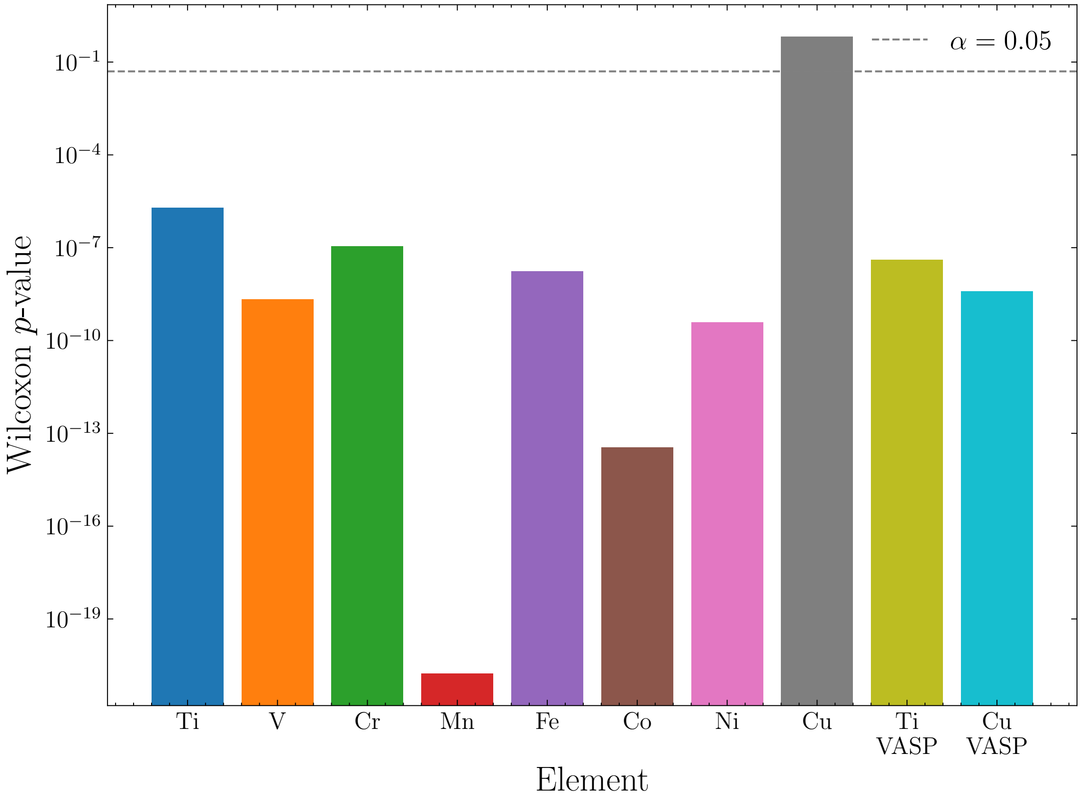


FIG. S6. Wilcoxon signed-rank test p-values comparing the performance of Tuned-UniversalXAS and ExpertXAS models across different elements. The test evaluates whether the mean squared error (MSE) per spectrum of the Tuned-UniversalXAS model is significantly smaller than that of the ExpertXAS model. Lower p-values provide stronger evidence that the Tuned-UniversalXAS model outperforms the ExpertXAS model. The dashed line represents the significance level $\alpha = 0.05$. For all elements except Cu/FEFF, p-values are well below this line, indicating that the probability of observing such a difference in performance by chance, assuming no true difference exists, is less than 5%.

[1] S. Ioffe and C. Szegedy, Batch normalization: Accelerating deep network training by reducing internal covariate shift, in *International conference on machine learning* (pmlr, 2015) pp. 448–456.

[2] P. Ramachandran, B. Zoph, and Q. V. Le, Searching for activation functions, arXiv preprint arXiv:1710.05941 (2017).

[3] G. E. Hinton, N. Srivastava, A. Krizhevsky, I. Sutskever, and R. R. Salakhutdinov, Improving neural networks by preventing co-adaptation of feature detectors, arXiv preprint arXiv:1207.0580 (2012).

[4] J. Bergstra, R. Bardenet, Y. Bengio, and B. Kégl, Algorithms for hyper-parameter optimization, Advances in neural information processing systems **24** (2011).

[5] T. Akiba, S. Sano, T. Yanase, T. Ohta, and M. Koyama, Optuna, Proceedings of the 25th ACM SIGKDD International Conference on Knowledge Discovery & Data Mining https://doi.org/10.1145/3292500.3330701 (2019).

[6] J. Behler, Atom-centered symmetry functions for constructing high-dimensional neural network potentials, J. Chem. Phys. **134**, 074106 (2011).

[7] L. Himanen, M. O. Jäger, E. V. Morooka, F. F. Canova, Y. S. Ranawat, D. Z. Gao, P. Rinke, and A. S. Foster, Dscribe: Library of descriptors for machine learning in materials science, Computer Physics Communications **247**, 106949 (2020).

[8] H. Kwon, W. Sun, T. Hsu, W. Jeong, F. Aydin, S. Sharma, F. Meng, M. R. Carbone, X. Chen, D. Lu, *et al.*, Harnessing neural networks for elucidating x-ray absorption structure–spectrum relationships in amorphous carbon, The Journal of Physical Chemistry C **127**, 16473 (2023).

[9] A. Ghose, M. Segal, F. Meng, Z. Liang, M. S. Hybertsen, X. Qu, E. Stavitski, S. Yoo, D. Lu, and M. R. Carbone, Uncertainty-aware predictions of molecular x-ray absorption spectra using neural network ensembles, Physical Review Research **5**, 013180 (2023).

[10] S. De, A. P. Bartók, G. Csányi, and M. Ceriotti, Comparing molecules and solids across structural and alchemical space, Physical Chemistry Chemical Physics **18**, 13754 (2016).

[11] Y. Bahri, E. Dyer, J. Kaplan, J. Lee, and U. Sharma, Explaining neural scaling laws, arXiv preprint arXiv:2102.06701 (2021).
